# Supplementary material for: Unified Graph Structured Models for Video Understanding
Source: arXiv:2103.15662 source file (2021-03-29)
Supplement: Supplementary file 1 [file compute_analysis.tex]

\section{Computation analysis}
\label{sec:supp_compute_analysis}

\begin{table*}[t]
	\centering
	\caption{Compute used by baseline and proposed models.
				 Our graph model is significantly more efficient than Non-local in the last layer of the backbone as it only passes messages to actor nodes, instead of all elements in the feature map.
				 Computation increases linearly with the number of frames processed, (and thus $\tau_c$), as the majority of compute is performed by the ResNet backbone.	
}
	\begin{tabular}{lcccc}
		\toprule
		Model & Frames & GFLOPs & Parameters ($\times10^6$) & SGCls R@20 \\ 
		\midrule
		SlowFast (ResNet 50)            						 & 32 &   74.18        &   34.6    &  48.9   \\
		Non-local in backbone           		  			   & 32 &   83.66         &   43.0    &  49.1   \\
		\midrule
		Spatial model, GAT, $\tau_c = 1$       		      & 32 &   74.41        &   36.5    & 51.1  \\
		Spatial model, Non-local, $\tau_c = 1$ 	        & 32 &   74.47        &   37.0    & 50.4 \\
		\midrule
		Spatio-temporal, GAT, $\tau_c = 3$     	        & 96   &   223.25      &   36.5   & 53.5  \\ 
		Spatio-temporal, GAT, $\tau_c = 5$     	        & 160 &   372.08      &   36.5   & 53.8  \\ 
		\bottomrule
	\end{tabular}
	\label{tab:compute}
\end{table*}

Table~\ref{tab:compute} shows the computation used by our models.
We measure compututation in terms of floating point operations (FLOPs), and GFLOPs denotes billions of FLOPs.

Our graph model is significantly more efficient than Non-local in the last layer of the backbone as it only passes messages to actor nodes, instead of all elements in the feature map.
Computation increases linearly with the number of frames processed, (and thus $\tau_c$), as the majority of compute is performed by the ResNet backbone
The computation required does not depend on $\tau_s$.

Note that our graph model adds neglible compute compared to the ResNet backbone.
In particular, the spatial model with GAT only adds 0.3\% more FLOPs to the ResNet backbone, while increasing SGCls R@20 by 4.5\%.

Finally, we note that compute is essentially identical for Action Genome and AVA models, as only the final ``read-out'' layer changes.
