# Supplementary material for: Unified Graph Structured Models for Video Understanding
Source: arXiv:2103.15662 source file (2021-03-29)
Supplement: Supplementary file 2 [file additional_qualitative.tex]

\section{Additional qualitative results}
\label{sec:supp_qualitative}

Please refer to the attached supplementary video for additional qualitative results on AVA, Action Genome and UCF101-24.

The codec used is ``H264 - MPEG-4 AVC'' and has been tested on ``VLC Media Player''.
